# Supplementary material for: Controlling the stoichiometry of the triangular lattice antiferromagnet Li$_{1+x}$Zn$_{2-y}$Mo$_3$O$_8$
Source: arXiv:1901.02171 source file (2019-01-08)
Supplement: Supplementary file 1 [file supplementary.pdf]

# Controlling the stoichiometry of the triangular lattice antiferromagnet $Li_{1+x}Zn_{2-y}Mo_3O_8$ – supplementary material

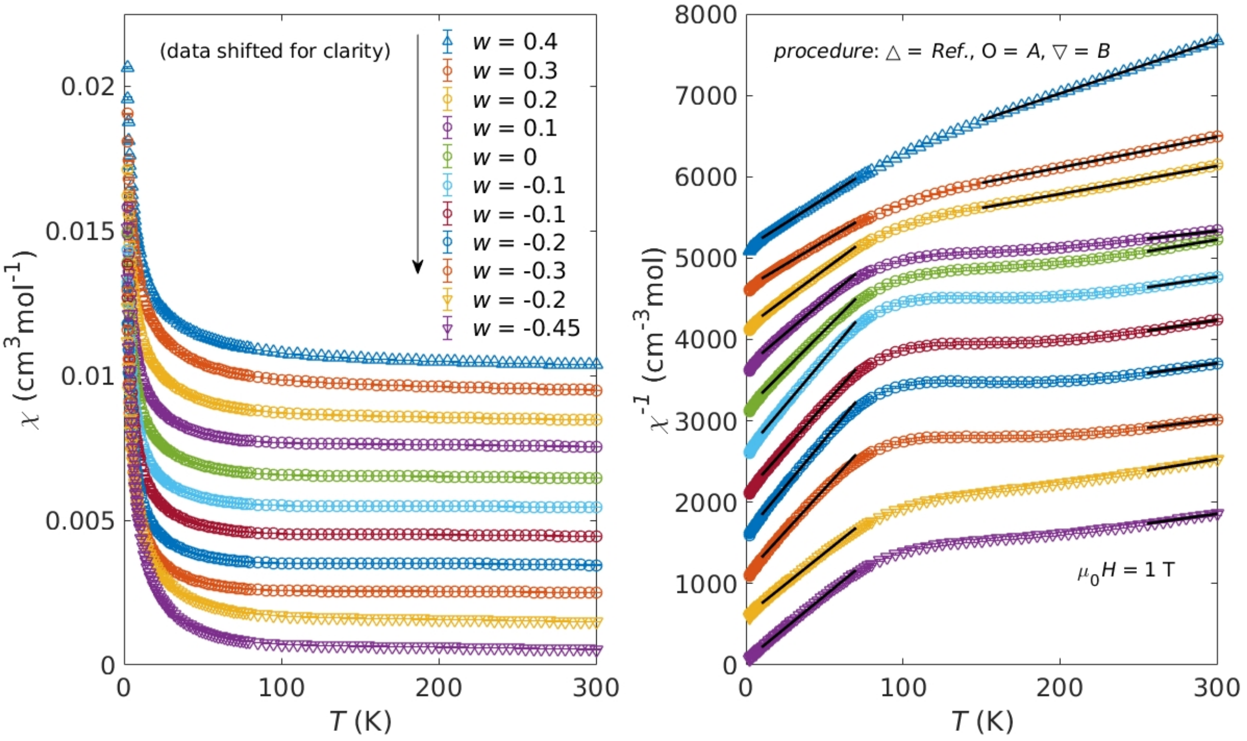


Figure 1: Magnetic susceptibility $\chi$ (left) and $\chi^{-1}$ (right) of all samples $w = -0.45$ – $0.4$. Two Curie-Weiss temperature regions are fitted using $\chi^{-1} = (T - \Theta)/C$. The fitting ranges of the low temperature region is $T = 10$ – $70$ K. For the high temperature region it is $T = 150$ – $300$ K and $T = 255$ – $300$ K for $w = 0.2$ – $0.4$ and $w = -0.45$ – $0.1$ samples, respectively. The results of the fitting, the effective magnetic moment sizes and Weiss temperatures are listed in Table 1

Table 1: Effective moment sizes and Weiss temperatures from the low and high temperature regions.

| *procedure* | *Ref* | *A* | *A* | *A* | *A* | *A* | *A* | *A* | *A* | *B* | *B* |
|---|---|---|---|---|---|---|---|---|---|---|---|
| $w$ | 0.4 | 0.3 | 0.2 | 0.1 | 0 | −0.1 | −0.1 | −0.2 | −0.3 | −0.2 | −0.45 |
| $\mu_{effLow}$ ($\mu_B$) | 0.807(1) | 0.832(1) | 0.748(2) | 0.699(2) | 0.642(2) | 0.591(2) | 0.607(2) | 0.588(2) | 0.616(2) | 0.719(2) | 0.712(2) |
| $\Theta_{Low}$ (K) | -9.9(1) | -11.5(1) | -10.0(2) | -10.0(2) | -7.4(2) | -5.3(2) | -5.2(2) | -4.9(2) | -5.3(2) | -6.6(2) | -3.8(2) |
| $\mu_{effHigh}$ ($\mu_B$) | 1.105(3) | 1.455(5) | 1.525(17) | 1.90(18) | 1.57(13) | 1.67(14) | 1.63(12) | 1.70(15) | 1.81(17) | 1.59(12) | 1.72(16) |
| $\Theta_{High}$ (K) | -109(2) | -227(3) | -320(12) | -530(150) | -390(110) | -490(130) | -440(110) | -500(130) | -530(160) | -340(100) | -390(130) |

Table 2: Structural parameters of $LiZn_2Mo_3O_8$ powder samples synthesized by the same method [13].

| Atom, $i$ | Site | $a_i/a$ | $b_i/b$ | $c_i/c$ | $U_{iso}$($\mathring{A}^2$) | occupancy |
|---|---|---|---|---|---|---|
| Ref. [17]: $Li_{1.0(1)}Zn_{1.8(1)}Mo_3O_8$, $a = 5.80163(3)$ Å, $c = 31.0738(2)$ Å. | | | | | | |
| Mo1 | 18h | 0.18504(8) | 0.81496(8) | 0.08393(4) | 0.0016(2) | 1 |
| O1 | 18h | 0.8445(2) | 0.1555(2) | 0.04850(6) | 0.0017(3) | 1 |
| O2 | 18h | 0.4920(2) | 0.5080(2) | 0.12438(7) | 0.0047(4) | 1 |
| O3 | 6c | 0 | 0 | 0.1185(1) | 0.0054(7) | 1 |
| O4 | 6c | 0 | 0 | 0.3715(1) | 0.0053(6) | 1 |
| Zn1 | 6c | 1/3 | 2/3 | −0.64176(7) | 0.0038(4) | 0.879(6) |
| Li1 | 6c | 1/3 | 2/3 | −0.64176(7) | 0.0038(4) | 0.00(4) |
| Zn2 | 6c | 0 | 0 | 0.1813(1) | 0.0038(4) | 0.679(5) |
| Li2 | 6c | 0 | 0 | 0.1813(1) | 0.0048(4) | 0.22(4) |
| Zn3 | 3a | 0 | 0 | 0 | 0.0038(4) | 0.265(7) |
| Li3 | 3a | 0 | 0 | 0 | 0.0038(4) | 0.58(6) |
| Zn4 | 6c | 0 | 0 | 0.5070(8) | 0.0038(4) | 0.065(4) |
| Li4 | 6c | 0 | 0 | 0.5070(8) | 0.0038(4) | 0.43(3) |
| Li5 | 6c | 2/3 | 1/3 | 0.08392(4) | 0.0038(4) | 0.09(3) |
| *procedure Ref*: $Li_{1.42(4)}Zn_{1.50(7)}Mo_3O_8$, $a = 5.7843(3)$ Å, $c = 31.053(2)$ Å | | | | | | |
| Mo1 | 18h | 0.18359(9) | 0.81641(9) | 0.08372(7) | 0.0053(3) | 1 |
| O1 | 18h | 0.8459(3) | 0.1541(3) | 0.04775(16) | 0.0061(4) | 1 |
| O2 | 18h | 0.4925(3) | 0.5075(3) | 0.12248(16) | 0.0061(4) | 1 |
| O3 | 6c | 0 | 0 | 0.1192(2) | 0.0061(4) | 1 |
| O4 | 6c | 0 | 0 | 0.3728(2) | 0.0061(4) | 1 |
| Zn1 | 6c | 1/3 | 2/3 | −0.64249(12) | 0.0074(9) | 0.850(4) |
| Li1 | 6c | 1/3 | 2/3 | −0.64249(12) | 0.0074(9) | 0.09(3) |
| Zn2 | 6c | 0 | 0 | 0.18212(17) | 0.0074(9) | 0.594(4) |
| Li2 | 6c | 0 | 0 | 0.18212(17) | 0.0074(9) | 0.41(3) |
| Zn3 | 3a | 0 | 0 | 0 | 0.0074(9) | 0.087(6) |
| Li3 | 3a | 0 | 0 | 0 | 0.0074(9) | 0.77(5) |
| Zn4 | 6c | 0 | 0 | 0.5104(11) | 0.0074(9) | 0.012(3) |
| Li4 | 6c | 0 | 0 | 0.5104(11) | 0.0074(9) | 0.51(3) |
| Li5 | 6c | 2/3 | 1/3 | 0.08392 | 0.0074(9) | 0.029(18) |
